# Supplementary material for: Multi-wavelength photometry during the 2018 superoutburst of the WZ Sge-type dwarf nova EG Cancri
Source: arXiv:2008.11871 ancillary file (2020-08-27)
Supplement: Supplementary file 1 [file si-egcnc-2018.pdf]

## References

Akitaya, Hiroshi, et al. 2014, in Proc. SPIE Vol. 9147 of Society of Photo-Optical Instrumentation Engineers (SPIE) Conference Series (p. 91474O)

Kotani, T., et al. 2005, Nuovo Cimento C Geophysics Space Physics C, 28, 755

Shimokawabe, Takashi, et al. 2008, in American Institute of Physics Conference Series, ed. M. Galassi, David Palmer, & Ed Fenimore Vol. 1000 of American Institute of Physics Conference Series (p. 543)

Yanagisawa, Kenshi, Kuroda, Daisuke, Yoshida, Michitoshi, Shimizu, Yasuhiro, Nagayama, Shogo, Toda, Hiroyuki, Ohta, Kouji, & Kawai, Nobuyuki 2010, in American Institute of Physics Conference Series, ed. Nobuyuki Kawai, & Shigehiro Nagataki Vol. 1279 of American Institute of Physics Conference Series (p. 466)

Yatsu, Yoichi, et al. 2007, Physica E Low-Dimensional Systems and Nanostructures, 40, 434

**Table E1.** Log of observations of the 2018 outburst in EG Cnc.

| Start* | End* | Mag† | Error‡ | $N$§ | Obs‖ | Band |
|---|---|---|---|---|---|---|
| 58396.9184 | 58396.9761 | 7.396 | 0.012 | 94 | Kis | $CV$ |
| 58397.4084 | 58397.6309 | 10.499 | 0.052 | 368 | Han | $V$ |
| 58397.4695 | 58397.6312 | 8.041 | 0.015 | 208 | DPV | $CV$ |
| 58397.5031 | 58397.6622 | 12.900 | 0.034 | 157 | NKa | $R_{\rm C}$ |
| 58397.5140 | 58397.5885 | 7.911 | 0.013 | 197 | CRI | $CV$ |
| 58397.5740 | 58397.6096 | 8.053 | 0.018 | 117 | Van | $CV$ |
| 58397.5998 | 58397.6623 | 10.609 | 0.026 | 90 | Trt | $V$ |
| 58397.6966 | 58397.7304 | 8.206 | 0.012 | 106 | Va2 | $CV$ |
| 58398.2327 | 58398.3370 | 13.527 | 0.033 | 258 | SCR | $r$ |
| 58398.2327 | 58398.3366 | 13.891 | 0.033 | 259 | SCR | $z$ |
| 58398.2327 | 58398.3370 | 13.735 | 0.033 | 256 | SCR | $i$ |
| 58398.2371 | 58398.3072 | 13.374 | 0.034 | 75 | MIT | $I_{\rm C}$ |
| 58398.2386 | 58398.3072 | 13.450 | 0.025 | 56 | MIT | $R_{\rm C}$ |
| 58398.2732 | 58398.3307 | 8.333 | 0.034 | 149 | Kis | $CV$ |
| 58398.2937 | 58398.3327 | 11.053 | 0.038 | 61 | Ioh | $V$ |
| 58398.3084 | 58398.3376 | 11.035 | 0.015 | 36 | OKU | $V$ |
| 58398.3944 | 58398.6062 | 11.270 | 0.067 | 209 | Han | $V$ |
| 58398.5992 | 58398.6416 | 13.682 | 0.028 | 41 | NKa | $R_{\rm C}$ |
| 58398.5003 | 58398.6073 | 8.674 | 0.026 | 280 | CRI | $CV$ |
| 58398.6217 | 58398.6515 | 8.888 | 0.026 | 40 | IMi | $CV$ |
| 58398.6426 | 58398.7307 | 8.855 | 0.030 | 244 | Van | $CV$ |
| 58398.9644 | 58399.0422 | 9.032 | 0.036 | 94 | SGE | $CV$ |
| 58399.1958 | 58399.3374 | 11.820 | 0.044 | 127 | KU1 | $V$ |
| 58399.2289 | 58399.3011 | 14.163 | 0.096 | 35 | MIT | $R_{\rm C}$ |
| 58399.2289 | 58399.3011 | 13.975 | 0.091 | 28 | MIT | $I_{\rm C}$ |
| 58399.2337 | 58399.3392 | 11.853 | 0.037 | 62 | OKU | $V$ |
| 58399.4030 | 58399.6334 | 11.858 | 0.074 | 229 | Han | $V$ |
| 58399.4890 | 58399.5995 | 9.158 | 0.045 | 291 | CRI | $CV$ |
| 58399.5742 | 58399.7306 | 8.969 | 0.153 | 674 | Van | $CV$ |
| 58399.9514 | 58400.0387 | 7.721 | 0.031 | 101 | SGE | $CV$ |
| 58400.1929 | 58400.3459 | 10.216 | 0.065 | 50 | KU1 | $V$ |
| 58400.2163 | 58400.3341 | 12.735 | 0.034 | 261 | SCR | $r$ |
| 58400.2163 | 58400.3341 | 13.091 | 0.033 | 278 | SCR | $z$ |
| 58400.2163 | 58400.3345 | 12.935 | 0.033 | 284 | SCR | $i$ |
| 58400.2281 | 58400.3413 | 10.233 | 0.042 | 117 | OKU | $V$ |
| 58400.2360 | 58400.3297 | 7.561 | 0.039 | 237 | Kis | $CV$ |
| 58400.2927 | 58400.3293 | 7.642 | 0.033 | 57 | Ioh | $CV$ |
| 58400.5251 | 58400.6683 | 12.433 | 0.044 | 120 | NKa | $R_{\rm C}$ |
| 58400.5538 | 58400.6212 | 7.493 | 0.050 | 178 | CRI | $CV$ |
| 58400.5732 | 58400.7302 | 7.573 | 0.046 | 450 | Van | $CV$ |
| 58400.6007 | 58400.6704 | 10.210 | 0.046 | 102 | Trt | $V$ |
| 58400.9449 | 58401.0486 | 7.360 | 0.049 | 121 | SGE | $CV$ |
| 58401.1925 | 58401.3493 | 9.995 | 0.056 | 74 | KU1 | $V$ |
| 58401.2357 | 58401.3339 | 7.332 | 0.042 | 220 | Kis | $CV$ |
| 58401.5337 | 58401.6548 | 7.559 | 0.048 | 286 | DPV | $CV$ |
| 58401.5437 | 58401.6388 | 12.406 | 0.045 | 83 | NKa | $R_{\rm C}$ |
| 58401.5738 | 58401.6993 | 7.543 | 0.044 | 415 | Van | $CV$ |
| 58401.5960 | 58401.6697 | 10.165 | 0.043 | 105 | Trt | $V$ |
| 58402.4788 | 58402.6709 | 12.453 | 0.041 | 157 | NKa | $R_{\rm C}$ |
| 58402.5014 | 58402.5535 | 10.118 | 0.043 | 53 | Han | $V$ |
| 58402.5819 | 58402.6605 | 10.227 | 0.031 | 113 | Trt | $V$ |
| 58403.4955 | 58403.6252 | 7.743 | 0.035 | 340 | CRI | $CV$ |

**Table E1.** Log of observations of the 2018 outburst in EG Cnc (continued).

| Start* | End* | Mag† | Error‡ | $N$§ | Obs‖ | Band |
|---|---|---|---|---|---|---|
| 58403.5013 | 58403.6597 | 7.690 | 0.035 | 366 | DPV | $CV$ |
| 58403.5823 | 58403.6503 | 10.302 | 0.035 | 193 | Trt | $V$ |
| 58404.2437 | 58404.3504 | 10.205 | 0.032 | 107 | KU1 | $V$ |
| 58404.2467 | 58404.3266 | 7.721 | 0.030 | 200 | OKU | $CV$ |
| 58404.5014 | 58404.6470 | 7.796 | 0.031 | 340 | DPV | $CV$ |
| 58404.6870 | 58404.7133 | 7.809 | 0.037 | 137 | Kai | $CV$ |
| 58404.9336 | 58405.0408 | 7.669 | 0.028 | 125 | SGE | $CV$ |
| 58405.5477 | 58405.6550 | 7.975 | 0.026 | 139 | DPV | $CV$ |
| 58405.5553 | 58405.7008 | 7.960 | 0.029 | 392 | Kai | $CV$ |
| 58405.6109 | 58405.6754 | 10.564 | 0.028 | 93 | Trt | $V$ |
| 58405.9676 | 58406.0504 | 7.796 | 0.026 | 115 | SGE | $CV$ |
| 58406.5083 | 58406.6790 | 12.910 | 0.027 | 162 | NKa | $R_C$ |
| 58406.5104 | 58406.6548 | 8.098 | 0.023 | 187 | DPV | $CV$ |
| 58406.6750 | 58406.7117 | 8.094 | 0.018 | 101 | Kai | $CV$ |
| 58406.9370 | 58407.0499 | 7.968 | 0.020 | 130 | SGE | $CV$ |
| 58407.2336 | 58407.3355 | 10.671 | 0.028 | 143 | KU1 | $V$ |
| 58407.3783 | 58407.4889 | 10.821 | 0.031 | 105 | Han | $V$ |
| 58407.4938 | 58407.4982 | 13.089 | 0.009 | 2 | NKa | $R_C$ |
| 58407.5702 | 58407.6404 | 11.046 | 0.034 | 101 | Trt | $V$ |
| 58407.5863 | 58407.6857 | 8.496 | 0.037 | 260 | Kai | $CV$ |
| 58407.9689 | 58408.0527 | 8.703 | 0.030 | 100 | SGE | $CV$ |
| 58408.4885 | 58408.6626 | 9.535 | 0.057 | 224 | DPV | $CV$ |
| 58408.5602 | 58408.6980 | 9.593 | 0.046 | 363 | Kai | $CV$ |
| 58408.5928 | 58408.6761 | 9.532 | 0.065 | 51 | Van | $CV$ |
| 58408.9711 | 58409.0341 | 9.921 | 0.032 | 100 | SGE | $CV$ |
| 58409.2151 | 58409.3471 | 15.280 | 0.059 | 33 | KU1 | $R_C$ |
| 58409.2456 | 58409.3345 | 15.083 | 0.043 | 28 | KU1 | $I_C$ |
| 58409.2470 | 58409.3479 | 12.999 | 0.051 | 32 | KU1 | $V$ |
| 58409.2537 | 58409.3397 | 15.666 | 0.067 | 27 | KU1 | $B$ |
| 58409.4798 | 58409.6563 | 10.894 | 0.072 | 121 | DPV | $CV$ |
| 58409.5972 | 58409.7019 | 10.948 | 0.058 | 127 | Kai | $CV$ |
| 58409.9383 | 58410.0439 | 11.295 | 0.058 | 115 | SGE | $CV$ |
| 58410.1940 | 58410.3454 | 15.689 | 0.083 | 15 | KU1 | $I_C$ |
| 58410.1954 | 58410.3469 | 14.027 | 0.118 | 14 | KU1 | $V$ |
| 58410.1961 | 58410.3476 | 16.829 | 0.174 | 5 | KU1 | $B$ |
| 58410.2392 | 58410.3332 | 16.074 | 0.066 | 7 | KU1 | $R_C$ |
| 58410.3083 | 58410.3244 | 13.996 | 0.098 | 10 | OKU | $V$ |
| 58410.9682 | 58411.0548 | 11.490 | 0.093 | 125 | SGE | $CV$ |
| 58411.1861 | 58411.2603 | 15.825 | 0.022 | 6 | KU1 | $I_C$ |
| 58411.1868 | 58411.2610 | 16.248 | 0.073 | 6 | KU1 | $R_C$ |
| 58411.1876 | 58411.2617 | 14.193 | 0.091 | 6 | KU1 | $V$ |
| 58411.2179 | 58411.2624 | 17.123 | 0.096 | 4 | KU1 | $B$ |
| 58411.3105 | 58411.3249 | 14.261 | 0.097 | 9 | OKU | $V$ |
| 58411.9283 | 58412.0543 | 11.486 | 0.082 | 98 | SGE | $CV$ |
| 58412.1823 | 58412.3366 | 11.541 | 0.307 | 195 | Kis | $CV$ |
| 58412.1933 | 58412.3050 | 15.155 | 0.095 | 35 | HHO | $J$ |
| 58412.1933 | 58412.3118 | 16.204 | 0.059 | 68 | HHO | $R_C$ |
| 58412.1960 | 58412.3509 | 14.130 | 0.096 | 62 | KU1 | $V$ |
| 58412.1975 | 58412.2124 | 15.742 | 0.130 | 2 | KU1 | $I_C$ |
| 58412.1997 | 58412.2145 | 17.206 | 0.261 | 2 | KU1 | $B$ |
| 58412.2036 | 58412.3134 | 14.566 | 0.141 | 32 | HHO | $K_S$ |
| 58412.2244 | 58412.3175 | 14.174 | 0.086 | 52 | OKU | $V$ |
| 58412.2254 | 58412.3082 | 16.193 | 0.074 | 28 | MIT | $R_C$ |

**Table E1.** Log of observations of the 2018 outburst in EG Cnc (continued).

| Start* | End* | Mag† | Error‡ | $N$§ | Obs‖ | Band |
|---|---|---|---|---|---|---|
| 58412.2270 | 58412.3075 | 15.708 | 0.074 | 22 | MIT | $I_C$ |
| 58412.2696 | 58412.3378 | 11.460 | 0.155 | 81 | Ioh | $CV$ |
| 58412.3431 | 58412.4313 | 16.053 | 0.043 | 53 | Hin | $R_C$ |
| 58412.9126 | 58413.0299 | 11.448 | 0.059 | 95 | SGE | $CV$ |
| 58413.1902 | 58413.3321 | 11.247 | 0.162 | 175 | Kis | $CV$ |
| 58413.2204 | 58413.3478 | 15.716 | 0.079 | 42 | KU1 | $I_C$ |
| 58413.2218 | 58413.3493 | 14.008 | 0.128 | 39 | KU1 | $V$ |
| 58413.2255 | 58413.3470 | 16.976 | 0.115 | 9 | KU1 | $B$ |
| 58413.2300 | 58413.3485 | 16.091 | 0.085 | 37 | KU1 | $R_C$ |
| 58414.1901 | 58414.2502 | 11.131 | 0.112 | 11 | KU1 | $CV$ |
| 58414.1901 | 58414.2495 | 15.504 | 0.044 | 4 | KU1 | $I_C$ |
| 58414.1909 | 58414.2502 | 16.007 | 0.075 | 4 | KU1 | $R_C$ |
| 58414.1927 | 58414.3065 | 11.185 | 0.317 | 156 | Ioh | $CV$ |
| 58414.1946 | 58414.2420 | 14.027 | 0.136 | 3 | KU1 | $V$ |
| 58415.9457 | 58416.0580 | 8.387 | 0.027 | 96 | SGE | $CV$ |
| 58416.1710 | 58416.3244 | 11.322 | 0.041 | 77 | OKU | $V$ |
| 58416.1739 | 58416.3570 | 13.741 | 0.061 | 62 | KU1 | $I_C$ |
| 58416.1753 | 58416.3555 | 11.307 | 0.053 | 61 | KU1 | $V$ |
| 58416.1760 | 58416.3533 | 13.856 | 0.049 | 52 | KU1 | $B$ |
| 58416.1776 | 58416.3548 | 13.734 | 0.051 | 59 | KU1 | $R_C$ |
| 58416.1784 | 58416.3402 | 8.657 | 0.061 | 271 | Kis | $CV$ |
| 58416.6257 | 58416.7454 | 9.319 | 0.045 | 146 | Van | $CV$ |
| 58416.9566 | 58417.0504 | 9.616 | 0.042 | 80 | SGE | $CV$ |
| 58417.1401 | 58417.2734 | 9.947 | 0.115 | 180 | Ioh | $CV$ |
| 58417.1679 | 58417.3536 | 14.978 | 0.074 | 54 | KU1 | $R_C$ |
| 58417.1701 | 58417.3499 | 14.836 | 0.067 | 60 | KU1 | $I_C$ |
| 58417.1714 | 58417.3111 | 12.644 | 0.066 | 79 | OKU | $V$ |
| 58417.1775 | 58417.3514 | 12.671 | 0.090 | 56 | KU1 | $V$ |
| 58417.1970 | 58417.3551 | 15.334 | 0.125 | 35 | KU1 | $B$ |
| 58417.3306 | 58417.3306 | 12.730 | – | 1 | Hsk | $V$ |
| 58417.4987 | 58417.6190 | 10.613 | 0.109 | 73 | BSM | $CV$ |
| 58418.9041 | 58419.0601 | 11.450 | 0.089 | 130 | SGE | $CV$ |
| 58419.1695 | 58419.3495 | 15.638 | 0.067 | 24 | KU1 | $I_C$ |
| 58419.1702 | 58419.3473 | 16.109 | 0.090 | 25 | KU1 | $R_C$ |
| 58419.1769 | 58419.3421 | 14.048 | 0.085 | 25 | KU1 | $V$ |
| 58419.2028 | 58419.3096 | 17.097 | 0.056 | 7 | KU1 | $B$ |
| 58419.2960 | 58419.3121 | 14.050 | 0.096 | 10 | OKU | $V$ |
| 58419.3304 | 58419.3304 | 14.206 | – | 1 | Ioh | $V$ |
| 58419.6255 | 58419.6916 | 10.685 | 0.114 | 101 | Van | $CV$ |
| 58420.1986 | 58420.3390 | 10.284 | 0.104 | 176 | Kis | $CV$ |
| 58420.2059 | 58420.2922 | 14.936 | 0.049 | 10 | KU1 | $I_C$ |
| 58420.2066 | 58420.2930 | 15.161 | 0.088 | 10 | KU1 | $R_C$ |
| 58420.2073 | 58420.2848 | 12.886 | 0.038 | 7 | KU1 | $V$ |
| 58420.2081 | 58420.2766 | 15.659 | 0.122 | 4 | KU1 | $B$ |
| 58420.2475 | 58420.2974 | 10.347 | 0.080 | 60 | Ioh | $CV$ |
| 58420.2958 | 58420.3030 | 13.121 | 0.015 | 5 | OKU | $V$ |
| 58420.3869 | 58420.6206 | 13.554 | 0.177 | 239 | Han | $V$ |
| 58420.4210 | 58420.6343 | 10.889 | 0.132 | 290 | CRI | $CV$ |
| 58421.2078 | 58421.3411 | 11.097 | 0.245 | 171 | Kis | $CV$ |
| 58421.3001 | 58421.3535 | 15.462 | 0.065 | 9 | KU1 | $I_C$ |
| 58421.3008 | 58421.3543 | 15.866 | 0.088 | 9 | KU1 | $R_C$ |
| 58421.3016 | 58421.3491 | 13.839 | 0.162 | 9 | KU1 | $V$ |

**Table E1.** Log of observations of the 2018 outburst in EG Cnc (continued).

| Start* | End* | Mag† | Error‡ | $N$§ | Obs‖ | Band |
|---|---|---|---|---|---|---|
| 58421.3023 | 58421.3498 | 16.821 | 0.094 | 6 | KU1 | $B$ |
| 58421.4245 | 58421.6037 | 11.103 | 0.105 | 246 | CRI | $CV$ |
| 58422.1824 | 58422.2879 | 11.218 | 0.193 | 138 | Ioh | $V$ |
| 58422.3340 | 58422.3412 | 10.937 | 0.008 | 5 | OKU | $V$ |
| 58422.5207 | 58422.6407 | 8.306 | 0.011 | 172 | Trt | $CV$ |
| 58422.5306 | 58422.5675 | 13.234 | 0.020 | 19 | NKa | $R_C$ |
| 58423.1095 | 58423.2836 | 11.384 | 0.085 | 240 | Ioh | $V$ |
| 58423.1622 | 58423.3190 | 11.422 | 0.058 | 144 | OKU | $V$ |
| 58423.2074 | 58423.3611 | 13.888 | 0.084 | 17 | KU1 | $I_C$ |
| 58423.2081 | 58423.3618 | 13.879 | 0.076 | 18 | KU1 | $R_C$ |
| 58423.2088 | 58423.3371 | 11.431 | 0.124 | 2 | KU1 | $V$ |
| 58423.2107 | 58423.3637 | 14.045 | 0.093 | 8 | KU1 | $B$ |
| 58423.5180 | 58423.5868 | 9.204 | 0.022 | 99 | Trt | $CV$ |
| 58424.1752 | 58424.3154 | 12.702 | 0.074 | 62 | OKU | $V$ |
| 58424.2296 | 58424.3506 | 12.826 | 0.127 | 103 | Ioh | $V$ |
| 58424.2312 | 58424.3479 | 15.445 | 0.191 | 92 | Ioh | $B$ |
| 58424.2762 | 58424.3334 | 14.933 | 0.038 | 20 | KU1 | $I_C$ |
| 58424.2770 | 58424.3304 | 15.092 | 0.047 | 19 | KU1 | $R_C$ |
| 58424.2777 | 58424.3311 | 12.799 | 0.053 | 18 | KU1 | $V$ |
| 58424.2784 | 58424.3318 | 15.477 | 0.062 | 18 | KU1 | $B$ |
| 58424.3988 | 58424.4976 | 13.074 | 0.130 | 99 | Han | $V$ |
| 58424.9924 | 58425.0506 | 11.192 | 0.040 | 50 | SGE | $CV$ |
| 58425.1755 | 58425.3425 | 10.612 | 0.155 | 198 | Kis | $CV$ |
| 58425.1887 | 58425.1947 | 15.532 | 0.038 | 2 | KU1 | $I_C$ |
| 58425.1895 | 58425.2013 | 15.938 | 0.039 | 3 | KU1 | $R_C$ |
| 58425.1902 | 58425.1961 | 13.835 | 0.048 | 2 | KU1 | $V$ |
| 58425.2245 | 58425.3511 | 13.988 | 0.332 | 184 | Ioh | $V$ |
| 58425.2858 | 58425.2858 | 13.785 | – | 1 | OKU | $V$ |
| 58425.4956 | 58425.5896 | 11.208 | 0.062 | 265 | Van | $CV$ |
| 58425.4987 | 58425.6128 | 15.899 | 0.057 | 29 | NKa | $R_C$ |
| 58426.0267 | 58426.0611 | 11.311 | 0.079 | 30 | SGE | $CV$ |
| 58426.2510 | 58426.2564 | 13.854 | 0.133 | 4 | OKU | $V$ |
| 58426.3827 | 58426.5142 | 13.981 | 0.123 | 101 | Han | $V$ |
| 58426.5765 | 58426.6415 | 15.784 | 0.138 | 21 | NKa | $R_C$ |
| 58427.1907 | 58427.3439 | 15.312 | 0.040 | 23 | KU1 | $I_C$ |
| 58427.1973 | 58427.3446 | 15.696 | 0.045 | 24 | KU1 | $R_C$ |
| 58427.1981 | 58427.3454 | 13.634 | 0.074 | 25 | KU1 | $V$ |
| 58427.1988 | 58427.3342 | 16.715 | 0.120 | 12 | KU1 | $B$ |
| 58427.2259 | 58427.3346 | 14.755 | 0.036 | 28 | HHO | $J$ |
| 58427.2259 | 58427.3448 | 15.669 | 0.042 | 94 | HHO | $R_C$ |
| 58427.2333 | 58427.3402 | 14.317 | 0.075 | 12 | HHO | $K_S$ |
| 58427.2623 | 58427.2679 | 15.660 | 0.104 | 4 | MIT | $R_C$ |
| 58427.2623 | 58427.2679 | 15.175 | 0.073 | 4 | MIT | $I_C$ |
| 58427.4146 | 58427.4321 | 13.538 | 0.091 | 19 | Han | $V$ |
| 58427.5275 | 58427.6458 | 15.843 | 0.055 | 90 | NKa | $R_C$ |
| 58427.9326 | 58428.0507 | 10.620 | 0.113 | 100 | SGE | $CV$ |
| 58428.4467 | 58428.6797 | 8.526 | 0.028 | 299 | DPV | $CV$ |
| 58428.5049 | 58428.6565 | 11.207 | 0.020 | 215 | Trt | $V$ |
| 58428.5378 | 58428.6412 | 13.339 | 0.018 | 86 | NKa | $R_C$ |
| 58428.5924 | 58428.7503 | 8.510 | 0.037 | 226 | Van | $CV$ |
| 58428.9767 | 58429.0609 | 11.372 | 0.029 | 86 | SGE | $V$ |
| 58429.1644 | 58429.1995 | 11.440 | 0.012 | 33 | OKU | $V$ |
| 58429.3203 | 58429.3619 | 14.027 | 0.027 | 15 | KU1 | $R_C$ |

**Table E1.** Log of observations of the 2018 outburst in EG Cnc (continued).

| Start* | End* | Mag† | Error‡ | $N$§ | Obs‖ | Band |
|---|---|---|---|---|---|---|
| 58429.3211 | 58429.3626 | 11.624 | 0.038 | 15 | KU1 | $V$ |
| 58429.3218 | 58429.3633 | 14.185 | 0.031 | 15 | KU1 | $B$ |
| 58429.3226 | 58429.3641 | 14.045 | 0.032 | 12 | KU1 | $I_{\rm C}$ |
| 58429.4544 | 58429.5697 | 14.232 | 0.042 | 24 | NKa | $R_{\rm C}$ |
| 58429.5359 | 58429.6668 | 9.557 | 0.056 | 90 | DPV | $CV$ |
| 58429.9442 | 58430.0621 | 12.658 | 0.050 | 93 | SGE | $V$ |
| 58429.9872 | 58430.0425 | 9.892 | 0.041 | 43 | SGE | $CV$ |
| 58430.1012 | 58430.1927 | 12.811 | 0.212 | 34 | Ioh | $V$ |
| 58430.1730 | 58430.2965 | 12.880 | 0.057 | 70 | OKU | $V$ |
| 58430.1759 | 58430.3590 | 15.005 | 0.067 | 61 | KU1 | $I_{\rm C}$ |
| 58430.1767 | 58430.3568 | 15.156 | 0.083 | 60 | KU1 | $R_{\rm C}$ |
| 58430.1774 | 58430.3605 | 12.925 | 0.086 | 61 | KU1 | $V$ |
| 58430.1781 | 58430.3612 | 15.657 | 0.139 | 57 | KU1 | $B$ |
| 58430.4880 | 58430.6807 | 10.879 | 0.067 | 132 | DPV | $CV$ |
| 58430.9967 | 58431.0437 | 13.903 | 0.059 | 50 | SGE | $V$ |
| 58431.4516 | 58431.6013 | 15.857 | 0.035 | 50 | NKa | $R_{\rm C}$ |
| 58431.5252 | 58431.6870 | 11.263 | 0.055 | 111 | DPV | $CV$ |
| 58431.9380 | 58432.0555 | 11.223 | 0.080 | 100 | SGE | $CV$ |
| 58432.4556 | 58432.6219 | 15.785 | 0.042 | 31 | NKa | $R_{\rm C}$ |
| 58432.9911 | 58433.0563 | 13.727 | 0.107 | 53 | SGE | $V$ |
| 58433.1503 | 58433.2596 | 13.881 | 0.176 | 61 | OKU | $V$ |
| 58433.2143 | 58433.2291 | 15.865 | 0.046 | 6 | KU1 | $R_{\rm C}$ |
| 58433.2165 | 58433.2314 | 15.477 | 0.053 | 6 | KU1 | $I_{\rm C}$ |
| 58433.2195 | 58433.3607 | 13.777 | 0.088 | 84 | KU1 | $V$ |
| 58433.2247 | 58433.2247 | 16.586 |  | 1 | KU1 | $B$ |
| 58433.2418 | 58433.3031 | 15.853 | 0.077 | 51 | MIT | $R_{\rm C}$ |
| 58433.2426 | 58433.3031 | 15.424 | 0.091 | 50 | MIT | $I_{\rm C}$ |
| 58433.2455 | 58433.3514 | 11.129 | 0.103 | 73 | Ioh | $CV$ |
| 58433.2628 | 58433.3083 | 15.121 | 0.044 | 32 | SCR | $z$ |
| 58433.2628 | 58433.3053 | 15.866 | 0.097 | 27 | SCR | $i$ |
| 58433.2634 | 58433.3494 | 16.037 | 0.135 | 36 | SCR | $r$ |
| 58433.3580 | 58433.3639 | 14.887 | 0.124 | 5 | HHO | $J$ |
| 58433.3581 | 58433.3699 | 16.365 | 0.475 | 9 | HHO | $R_{\rm C}$ |
| 58433.3675 | 58433.3675 | 14.698 | – | 1 | HHO | $K_{\rm S}$ |
| 58433.4475 | 58433.4769 | 11.175 | 0.115 | 20 | DPV | $CV$ |
| 58433.4663 | 58433.6513 | 15.811 | 0.054 | 28 | NKa | $R_{\rm C}$ |
| 58434.3219 | 58434.3362 | 13.573 | 0.044 | 8 | OKU | $V$ |
| 58434.3262 | 58434.3559 | 15.204 | 0.047 | 5 | KU1 | $I_{\rm C}$ |
| 58434.3269 | 58434.3625 | 15.557 | 0.055 | 6 | KU1 | $R_{\rm C}$ |
| 58434.3277 | 58434.3514 | 13.518 | 0.035 | 4 | KU1 | $V$ |
| 58434.3284 | 58434.3343 | 16.585 | 0.167 | 2 | KU1 | $B$ |
| 58434.4741 | 58434.6831 | 9.390 | 0.569 | 143 | DPV | $CV$ |
| 58434.9472 | 58435.0538 | 11.040 | 0.012 | 110 | SGE | $V$ |
| 58435.4788 | 58435.6583 | 8.992 | 0.056 | 123 | DPV | $CV$ |
| 58435.9479 | 58436.0598 | 12.054 | 0.062 | 112 | SGE | $V$ |
| 58436.1837 | 58436.3231 | 14.584 | 0.057 | 40 | KU1 | $I_{\rm C}$ |
| 58436.1873 | 58436.3179 | 14.833 | 0.065 | 19 | KU1 | $B$ |
| 58436.1874 | 58436.3476 | 14.622 | 0.063 | 44 | KU1 | $R_{\rm C}$ |
| 58436.1940 | 58436.3483 | 12.256 | 0.051 | 39 | KU1 | $V$ |

**Table E1.** Log of observations of the 2018 outburst in EG Cnc (continued).

| Start* | End* | Mag† | Error‡ | $N$§ | Obs‖ | Band |
|---|---|---|---|---|---|---|
| 58436.4303 | 58436.6097 | 14.950 | 0.098 | 44 | NKa | $R_C$ |
| 58436.5763 | 58436.7408 | 10.395 | 0.086 | 303 | Van | $CV$ |
| 58436.9337 | 58437.0706 | 13.644 | 0.103 | 140 | SGE | $V$ |
| 58437.1738 | 58437.1899 | 13.617 | 0.072 | 10 | OKU | $V$ |
| 58437.1840 | 58437.2466 | 13.720 | 0.247 | 87 | Ioh | $V$ |
| 58437.1873 | 58437.3665 | 15.777 | 0.063 | 61 | KU1 | $R_C$ |
| 58437.2058 | 58437.3613 | 13.701 | 0.081 | 52 | KU1 | $V$ |
| 58437.2132 | 58437.3657 | 15.431 | 0.064 | 38 | KU1 | $I_C$ |
| 58437.2288 | 58437.3635 | 16.646 | 0.044 | 8 | KU1 | $B$ |
| 58437.9141 | 58438.0601 | 13.923 | 0.088 | 150 | SGE | $V$ |
| 58438.1516 | 58438.2110 | 15.535 | 0.074 | 149 | SCR | $z$ |
| 58438.1516 | 58438.2110 | 15.571 | 0.083 | 147 | SCR | $i$ |
| 58438.1520 | 58438.2110 | 15.661 | 0.113 | 122 | SCR | $r$ |
| 58438.1709 | 58438.2445 | 13.316 | 0.192 | 99 | Ioh | $V$ |
| 58438.1800 | 58438.3724 | 13.355 | 0.052 | 271 | KU1 | $V$ |
| 58438.2318 | 58438.2968 | 14.760 | 0.030 | 25 | HHO | $J$ |
| 58438.2319 | 58438.2968 | 15.529 | 0.043 | 55 | HHO | $R_C$ |
| 58438.2390 | 58438.2883 | 14.544 | 0.057 | 7 | HHO | $K_S$ |
| 58438.2546 | 58438.3041 | 15.463 | 0.061 | 20 | MIT | $R_C$ |
| 58438.2546 | 58438.3041 | 15.102 | 0.074 | 20 | MIT | $I_C$ |
| 58438.9079 | 58439.0577 | 13.790 | 0.102 | 114 | SGE | $V$ |
| 58439.5103 | 58439.6612 | 11.115 | 0.108 | 216 | Trt | $CV$ |
| 58439.5557 | 58439.7409 | 11.111 | 0.085 | 246 | Van | $CV$ |
| 58440.1770 | 58440.3680 | 15.683 | 0.070 | 64 | KU1 | $R_C$ |
| 58440.1778 | 58440.3687 | 13.614 | 0.086 | 57 | KU1 | $V$ |
| 58440.1778 | 58440.3658 | 15.348 | 0.073 | 32 | KU1 | $I_C$ |
| 58440.1814 | 58440.3635 | 16.614 | 0.112 | 19 | KU1 | $B$ |
| 58440.2972 | 58440.3133 | 13.553 | 0.024 | 10 | OKU | $V$ |
| 58440.6372 | 58440.7367 | 8.723 | 0.112 | 125 | Van | $CV$ |
| 58440.9553 | 58441.0735 | 11.164 | 0.018 | 110 | SGE | $V$ |
| 58441.4124 | 58441.6248 | 13.904 | 0.086 | 126 | NKa | $R_C$ |
| 58441.5158 | 58441.6946 | 9.044 | 0.066 | 229 | IMi | $CV$ |
| 58441.6381 | 58441.6730 | 9.110 | 0.023 | 53 | Van | $CV$ |
| 58442.2057 | 58442.2683 | 12.375 | 0.027 | 36 | OKU | $V$ |
| 58442.3018 | 58442.3662 | 12.531 | 0.049 | 92 | KU1 | $V$ |
| 58442.9025 | 58443.0641 | 13.892 | 0.111 | 162 | SGE | $V$ |
| 58443.0910 | 58443.0910 | 14.286 | – | 1 | Ioh | $V$ |
| 58443.2212 | 58443.2538 | 15.591 | 0.054 | 9 | KU1 | $I_C$ |
| 58443.2219 | 58443.2545 | 15.991 | 0.061 | 12 | KU1 | $R_C$ |
| 58443.2226 | 58443.2552 | 13.995 | 0.073 | 10 | KU1 | $V$ |
| 58443.2248 | 58443.2545 | 16.878 | 0.142 | 6 | KU1 | $B$ |
| 58443.2570 | 58443.3702 | 11.039 | 0.092 | 155 | KU1 | $CV$ |
| 58443.2717 | 58443.2878 | 13.848 | 0.092 | 10 | OKU | $V$ |
| 58443.9675 | 58444.0757 | 14.037 | 0.152 | 116 | SGE | $V$ |
| 58445.1926 | 58445.1926 | 13.826 | – | 1 | Ioh | $V$ |
| 58445.2061 | 58445.2968 | 15.844 | 0.064 | 12 | KU1 | $R_C$ |
| 58445.2083 | 58445.2857 | 15.528 | 0.105 | 4 | KU1 | $I_C$ |
| 58445.2098 | 58445.2975 | 13.720 | 0.049 | 9 | KU1 | $V$ |
| 58445.2789 | 58445.3012 | 16.639 | 0.057 | 3 | KU1 | $B$ |
| 58445.2807 | 58445.2968 | 13.703 | 0.062 | 10 | OKU | $V$ |
| 58445.3570 | 58445.3669 | 10.846 | 0.063 | 15 | KU1 | $CV$ |
| 58445.3714 | 58445.5014 | 11.609 | 0.193 | 62 | CRI | $CV$ |
| 58446.1059 | 58446.3286 | 13.978 | 0.222 | 86 | OKU | $V$ |

**Table E1.** Log of observations of the 2018 outburst in EG Cnc (continued).

| Start* | End* | Mag† | Error‡ | $N$§ | Obs‖ | Band |
|---|---|---|---|---|---|---|
| 58446.2157 | 58446.3672 | 13.862 | 0.143 | 28 | KU1 | $V$ |
| 58446.2334 | 58446.3680 | 16.012 | 0.123 | 39 | KU1 | $R_C$ |
| 58446.2356 | 58446.3643 | 15.608 | 0.088 | 27 | KU1 | $I_C$ |
| 58446.2408 | 58446.3269 | 16.856 | 0.076 | 10 | KU1 | $B$ |
| 58446.3240 | 58446.3240 | 14.036 | – | 1 | Ioh | $V$ |
| 58446.4170 | 58446.5009 | 11.834 | 0.125 | 39 | CRI | $CV$ |
| 58446.4382 | 58446.6691 | 14.515 | 0.233 | 230 | Han | $V$ |
| 58447.1826 | 58447.3558 | 11.218 | 0.200 | 164 | Ioh | $CV$ |
| 58447.2224 | 58447.3620 | 15.897 | 0.124 | 20 | KU1 | $I_C$ |
| 58447.2232 | 58447.3628 | 16.423 | 0.128 | 22 | KU1 | $R_C$ |
| 58447.2254 | 58447.3650 | 14.375 | 0.168 | 13 | KU1 | $V$ |
| 58447.2261 | 58447.3568 | 17.441 | 0.154 | 12 | KU1 | $B$ |
| 58447.2376 | 58447.3378 | 14.461 | 0.197 | 57 | OKU | $V$ |
| 58447.3868 | 58447.4139 | 14.619 | 0.265 | 23 | Han | $V$ |
| 58448.1639 | 58448.3435 | 14.406 | 0.206 | 21 | KU1 | $V$ |
| 58448.1639 | 58448.3672 | 15.952 | 0.212 | 20 | KU1 | $I_C$ |
| 58448.1647 | 58448.3234 | 16.418 | 0.085 | 12 | KU1 | $R_C$ |
| 58448.1676 | 58448.3264 | 17.139 | 0.218 | 5 | KU1 | $B$ |
| 58448.2340 | 58448.3397 | 14.435 | 0.280 | 58 | OKU | $V$ |
| 58448.2741 | 58448.2741 | 15.920 | – | 1 | Ioh | $I_C$ |
| 58448.2769 | 58448.2769 | 14.316 | – | 1 | Ioh | $V$ |
| 58450.1068 | 58450.2101 | 13.086 | 0.278 | 97 | Ioh | $V$ |
| 58450.2408 | 58450.3447 | 12.704 | 0.058 | 58 | OKU | $V$ |
| 58450.2411 | 58450.3830 | 14.821 | 0.089 | 19 | KU1 | $I_C$ |
| 58450.2418 | 58450.3808 | 14.952 | 0.088 | 20 | KU1 | $R_C$ |
| 58450.2455 | 58450.3845 | 12.674 | 0.128 | 19 | KU1 | $V$ |
| 58450.2462 | 58450.3284 | 15.405 | 0.101 | 6 | KU1 | $B$ |
| 58451.1993 | 58451.3671 | 11.200 | 0.040 | 220 | OKU | $V$ |
| 58451.2488 | 58451.3296 | 13.676 | 0.071 | 49 | HHO | $R_C$ |
| 58451.2844 | 58451.3764 | 13.608 | 0.035 | 22 | KU1 | $I_C$ |
| 58451.2852 | 58451.3741 | 13.614 | 0.033 | 27 | KU1 | $R_C$ |
| 58451.2859 | 58451.3393 | 11.206 | 0.018 | 16 | KU1 | $V$ |
| 58451.2866 | 58451.3786 | 13.809 | 0.036 | 22 | KU1 | $B$ |
| 58451.4067 | 58451.6697 | 11.478 | 0.097 | 264 | Han | $V$ |
| 58451.4413 | 58451.6539 | 8.794 | 0.058 | 304 | Trt | $CV$ |
| 58451.6119 | 58451.7216 | 14.026 | 0.045 | 86 | NKa | $R_C$ |
| 58451.6667 | 58451.7072 | 11.796 | 0.039 | 10 | DPV | $V$ |
| 58451.6682 | 58451.7087 | 14.034 | 0.039 | 10 | DPV | $R_C$ |
| 58451.6697 | 58451.7102 | 14.022 | 0.093 | 10 | DPV | $I_C$ |
| 58452.0960 | 58452.2082 | 12.272 | 0.117 | 154 | Ioh | $V$ |
| 58452.1070 | 58452.3426 | 12.377 | 0.118 | 122 | OKU | $V$ |
| 58452.1919 | 58452.3622 | 14.790 | 0.107 | 31 | KU1 | $R_C$ |
| 58452.1926 | 58452.3658 | 12.427 | 0.151 | 32 | KU1 | $V$ |
| 58452.1933 | 58452.3636 | 14.975 | 0.125 | 28 | KU1 | $B$ |
| 58452.1941 | 58452.3585 | 14.745 | 0.125 | 28 | KU1 | $I_C$ |
| 58452.4583 | 58452.6379 | 10.458 | 0.095 | 123 | DPV | $CV$ |
| 58452.6467 | 58452.6737 | 13.300 | 0.117 | 7 | DPV | $V$ |
| 58453.1315 | 58453.3018 | 16.024 | 0.075 | 14 | KU1 | $I_C$ |
| 58453.1323 | 58453.3025 | 16.408 | 0.089 | 15 | KU1 | $R_C$ |
| 58453.1330 | 58453.3062 | 14.340 | 0.194 | 18 | KU1 | $V$ |
| 58453.1412 | 58453.2391 | 14.204 | 0.165 | 18 | OKU | $V$ |
| 58453.1946 | 58453.2746 | 17.098 | 0.048 | 3 | KU1 | $B$ |

**Table E1.** Log of observations of the 2018 outburst in EG Cnc (continued).

| Start* | End* | Mag† | Error‡ | $N$§ | Obs‖ | Band |
|---|---|---|---|---|---|---|
| 58453.2405 | 58453.2405 | 16.160 | – | 1 | Ioh | $I_C$ |
| 58453.2412 | 58453.2412 | 14.316 | – | 1 | Ioh | $V$ |
| 58453.4810 | 58453.7038 | 11.841 | 0.096 | 150 | DPV | $CV$ |
| 58453.5874 | 58453.6202 | 11.681 | 0.058 | 37 | Van | $CV$ |
| 58453.6001 | 58453.7183 | 16.501 | 0.092 | 42 | NKa | $R_C$ |
| 58454.1412 | 58454.3734 | 14.576 | 0.213 | 15 | KU1 | $V$ |
| 58454.1419 | 58454.1894 | 17.277 | 0.166 | 3 | KU1 | $B$ |
| 58454.1419 | 58454.3742 | 16.652 | 0.134 | 19 | KU1 | $R_C$ |
| 58454.1590 | 58454.3735 | 16.275 | 0.076 | 9 | KU1 | $I_C$ |
| 58454.2180 | 58454.3447 | 14.557 | 0.124 | 54 | OKU | $V$ |
| 58457.5481 | 58457.7090 | 12.208 | 0.064 | 98 | NKa | $CV$ |
| 58458.3418 | 58458.3561 | 14.811 | 0.181 | 4 | OKU | $V$ |
| 58458.6297 | 58458.7151 | 12.244 | 0.053 | 74 | NKa | $CV$ |
| 58460.5655 | 58460.6288 | 12.256 | 0.085 | 69 | Van | $CV$ |
| 58461.5143 | 58461.5681 | 12.233 | 0.059 | 37 | NKa | $CV$ |
| 58461.8687 | 58462.0867 | 14.872 | 0.222 | 221 | SGE | $V$ |
| 58462.2354 | 58462.2659 | 14.739 | 0.098 | 9 | OKU | $V$ |
| 58463.2111 | 58463.3167 | 15.042 | 0.167 | 45 | OKU | $V$ |
| 58463.2782 | 58463.3791 | 16.591 | 0.060 | 23 | KU1 | $I_C$ |
| 58463.2789 | 58463.3844 | 15.042 | 0.093 | 24 | KU1 | $V$ |
| 58463.8333 | 58464.0519 | 14.955 | 0.164 | 224 | SGE | $V$ |
| 58464.9764 | 58465.0765 | 15.099 | 0.130 | 116 | SGE | $V$ |
| 58465.2930 | 58465.3091 | 14.905 | 0.099 | 10 | OKU | $V$ |
| 58465.3245 | 58465.3407 | 16.398 | 0.093 | 10 | OKU | $I_C$ |
| 58466.0809 | 58466.1003 | 16.746 | 0.126 | 13 | SCR | $z$ |
| 58466.0816 | 58466.1003 | 17.260 | 0.160 | 11 | SCR | $r$ |
| 58466.0816 | 58466.0996 | 16.925 | 0.103 | 15 | SCR | $i$ |
| 58466.2301 | 58466.2462 | 15.036 | 0.139 | 10 | OKU | $V$ |
| 58466.2489 | 58466.2750 | 16.454 | 0.088 | 5 | OKU | $I_C$ |
| 58468.1938 | 58468.1938 | 15.206 | – | 1 | Ioh | $V$ |
| 58468.1951 | 58468.1951 | 17.570 | – | 1 | Ioh | $I_C$ |
| 58468.2428 | 58468.2536 | 15.046 | 0.129 | 6 | OKU | $V$ |
| 58468.2591 | 58468.2753 | 16.617 | 0.084 | 10 | OKU | $I_C$ |
| 58468.3566 | 58468.3832 | 16.740 | 0.088 | 4 | KU1 | $I_C$ |
| 58468.3573 | 58468.3840 | 17.270 | 0.144 | 4 | KU1 | $R_C$ |
| 58468.3580 | 58468.3847 | 15.411 | 0.354 | 3 | KU1 | $V$ |
| 58468.3587 | 58468.3765 | 18.012 | 0.013 | 2 | KU1 | $B$ |
| 58469.5768 | 58469.6958 | 12.577 | 0.071 | 100 | NKa | $CV$ |
| 58470.2250 | 58470.2394 | 15.191 | 0.261 | 9 | OKU | $V$ |
| 58470.2413 | 58470.2574 | 16.689 | 0.105 | 10 | OKU | $I_C$ |
| 58471.2810 | 58471.2918 | 15.236 | 0.096 | 7 | OKU | $V$ |
| 58471.2937 | 58471.3098 | 16.642 | 0.090 | 10 | OKU | $I_C$ |
| 58471.3499 | 58471.3766 | 17.012 | 0.104 | 4 | KU1 | $I_C$ |
| 58471.3506 | 58471.3773 | 17.445 | 0.184 | 4 | KU1 | $R_C$ |
| 58471.3513 | 58471.3780 | 15.233 | 0.163 | 3 | KU1 | $V$ |
| 58471.3565 | 58471.3743 | 17.367 | 0.447 | 2 | KU1 | $B$ |
| 58471.6244 | 58471.7156 | 12.513 | 0.060 | 62 | DPV | $CV$ |
| 58473.3469 | 58473.3825 | 17.254 | 0.165 | 5 | KU1 | $R_C$ |
| 58473.3477 | 58473.3743 | 15.271 | 0.402 | 4 | KU1 | $V$ |
| 58473.3551 | 58473.3818 | 16.765 | 0.123 | 4 | KU1 | $I_C$ |
| 58473.3573 | 58473.3840 | 17.759 | 0.168 | 2 | KU1 | $B$ |
| 58476.2913 | 58476.3057 | 16.937 | 0.156 | 9 | OKU | $I_C$ |

**Table E1.** Log of observations of the 2018 outburst in EG Cnc (continued).

| Start* | End* | Mag† | Error‡ | $N$§ | Obs‖ | Band |
|---|---|---|---|---|---|---|
| 58476.3077 | 58476.3238 | 15.096 | 0.115 | 8 | OKU | $V$ |
| 58477.0342 | 58477.0342 | 17.449 | – | 1 | SCR | $r$ |
| 58477.0342 | 58477.0342 | 17.411 | – | 1 | SCR | $i$ |
| 58477.3423 | 58477.3868 | 16.707 | 0.198 | 6 | KU1 | $R_C$ |
| 58477.3431 | 58477.3787 | 16.014 | 0.174 | 4 | KU1 | $I_C$ |
| 58477.3445 | 58477.3920 | 14.725 | 0.197 | 5 | KU1 | $V$ |
| 58477.3616 | 58477.3764 | 16.630 | 0.162 | 2 | KU1 | $B$ |
| 58482.1464 | 58482.1583 | 17.091 | 0.124 | 3 | KU1 | $I_C$ |
| 58482.1471 | 58482.1531 | 17.839 | 0.083 | 2 | KU1 | $R_C$ |
| 58482.1478 | 58482.1538 | 15.215 | 0.085 | 2 | KU1 | $V$ |
| 58482.2722 | 58482.3728 | 13.533 | 0.697 | 84 | Ioh | $CV$ |
| 58483.1977 | 58483.3709 | 12.764 | 0.248 | 122 | Ioh | $CV$ |
| 58484.3815 | 58484.3874 | 17.302 | 0.428 | 2 | KU1 | $I_C$ |
| 58484.3822 | 58484.3882 | 17.852 | 0.057 | 2 | KU1 | $R_C$ |
| 58484.3859 | 58484.3859 | 15.278 | – | 1 | KU1 | $V$ |
| 58485.2108 | 58485.3746 | 12.966 | 0.257 | 141 | Ioh | $CV$ |
| 58486.0652 | 58486.0896 | 15.698 | 0.201 | 29 | SGE | $V$ |
| 58487.3433 | 58487.3611 | 17.638 | 0.008 | 3 | KU1 | $R_C$ |
| 58487.3440 | 58487.3559 | 17.232 | 0.075 | 2 | KU1 | $I_C$ |
| 58487.3455 | 58487.3692 | 15.558 | 0.250 | 3 | KU1 | $V$ |
| 58488.2145 | 58488.3743 | 13.245 | 0.373 | 137 | Ioh | $CV$ |
| 58491.3686 | 58491.3834 | 17.444 | 0.722 | 2 | KU1 | $I_C$ |
| 58491.3700 | 58491.3849 | 14.552 | 0.171 | 2 | KU1 | $V$ |
| 58491.3841 | 58491.3841 | 17.301 | – | 1 | KU1 | $R_C$ |
| 58493.3573 | 58493.3573 | 15.687 | – | 1 | KU1 | $V$ |
| 58493.3596 | 58493.3596 | 18.456 | – | 1 | KU1 | $R_C$ |
| 58493.3603 | 58493.3603 | 17.361 | – | 1 | KU1 | $I_C$ |
| 58498.2807 | 58498.2853 | 17.763 | 0.238 | 2 | KU1 | $I_C$ |
| 58498.2822 | 58498.2822 | 16.017 | – | 1 | KU1 | $V$ |
| 58506.2924 | 58506.3337 | 17.204 | 0.242 | 5 | KU1 | $I_C$ |
| 58506.3076 | 58506.3558 | 15.203 | 0.241 | 6 | KU1 | $V$ |

*BJD − 2400000.0.

†Mean magnitude.

‡$1\sigma$ of mean magnitude.

§Number of observations.

‖Observer's code: Kis (Seiichiro Kiyota), DPV (Pavol A. Dubovsky), Van & Va2 (Tonny Vanmunster), IMi (Ian Miller), SGE (Sergey Yu. Shugarov), Ioh (Hiroshi Itoh), OKU (Osaka Kyoiku Univ. team), Kai (Kiyoshi Kasai), KU1 (Kyoto U. team), BSM (Stephen M. Brincat), Trt (Tamás Tordai), NKa (Natalia Katysheva), Han (Arto Oksanen), Hsk (Kenji Hirosawa), SCR (Saitama U. team), MIT (MITSuME at Tokyo Institute of Technology (Akeno & Okayama) Kotani et al. (2005); Yatsu et al. (2007); Shimokawabe et al. (2008); Yanagisawa et al. (2010)), HHO (HONIR at Higashi-Hiroshima Observatory Akitaya et al. (2014)), Hin (HinOTORI at Ali Observatory, Western Tibet, China), CRI (Crimean Astrophysical Observatory).

**Table E2.** Times of superhump maxima in the 2018 outburst of EG Cnc.

| $E$ | Max[†] | Error | $O-C$[‡] | $N$[§] |
|---|---|---|---|---|
| -25 | 58398.4621 | 0.0016 | -0.0078 | 50 |
| -24 | 58398.5236 | 0.0015 | -0.0068 | 49 |
| -16 | 58399.0046 | 0.0005 | -0.0084 | 58 |
| -12 | 58399.2490 | 0.0006 | -0.0053 | 71 |
| -11 | 58399.3113 | 0.0005 | -0.0033 | 74 |
| -8 | 58399.4907 | 0.0005 | -0.0049 | 50 |
| -7 | 58399.5532 | 0.0010 | -0.0028 | 72 |
| -6 | 58399.6105 | 0.0004 | -0.0059 | 233 |
| -5 | 58399.6700 | 0.0004 | -0.0067 | 287 |
| 0 | 58399.9709 | 0.0008 | -0.0074 | 52 |
| 4 | 58400.2142 | 0.0012 | -0.0054 | 85 |
| 5 | 58400.2755 | 0.0006 | -0.0045 | 276 |
| 6 | 58400.3373 | 0.0007 | -0.0030 | 161 |
| 10 | 58400.5806 | 0.0006 | -0.0011 | 149 |
| 11 | 58400.6414 | 0.0002 | -0.0006 | 267 |
| 12 | 58400.7028 | 0.0003 | 0.0004 | 99 |
| 16 | 58400.9438 | 0.0007 | 0.0001 | 30 |
| 17 | 58401.0039 | 0.0003 | -0.0001 | 57 |
| 22 | 58401.3047 | 0.0004 | -0.0010 | 108 |
| 25 | 58401.4890 | 0.0002 | 0.0023 | 94 |
| 26 | 58401.5478 | 0.0003 | 0.0008 | 131 |
| 27 | 58401.6076 | 0.0002 | 0.0003 | 367 |
| 28 | 58401.6690 | 0.0002 | 0.0014 | 211 |
| 44 | 58402.6343 | 0.0004 | 0.0013 | 105 |
| 59 | 58403.5373 | 0.0003 | -0.0007 | 113 |
| 60 | 58403.5977 | 0.0003 | -0.0006 | 234 |
| 61 | 58403.6590 | 0.0009 | 0.0003 | 115 |
| 71 | 58404.2631 | 0.0005 | 0.0011 | 154 |
| 72 | 58404.3223 | 0.0004 | -0.0000 | 116 |
| 75 | 58404.5091 | 0.0007 | 0.0018 | 73 |
| 76 | 58404.5642 | 0.0004 | 0.0005 | 112 |
| 77 | 58404.6176 | 0.0003 | -0.0004 | 111 |
| 83 | 58404.9868 | 0.0005 | 0.0008 | 56 |
| 94 | 58405.6495 | 0.0004 | -0.0001 | 67 |
| 109 | 58406.5557 | 0.0007 | 0.0010 | 32 |
| 110 | 58406.6147 | 0.0005 | -0.0003 | 57 |
| 121 | 58407.2788 | 0.0009 | 0.0001 | 68 |
| 124 | 58407.4619 | 0.0009 | 0.0022 | 47 |
| 127 | 58407.6395 | 0.0005 | -0.0011 | 159 |
| 133 | 58408.0040 | 0.0006 | 0.0013 | 57 |
| 142 | 58408.5474 | 0.0006 | 0.0017 | 99 |
| 143 | 58408.6067 | 0.0006 | 0.0007 | 218 |
| 144 | 58408.6660 | 0.0007 | -0.0003 | 167 |
| 181 | 58410.9876 | 0.0010 | -0.0318 | 69 |
| 182 | 58411.0366 | 0.0023 | -0.0431 | 55 |
| 199 | 58411.9535 | 0.0015 | -0.0312 | 36 |
| 200 | 58412.0128 | 0.0015 | -0.0323 | 37 |
| 206 | 58412.3767 | 0.0034 | -0.0303 | 27 |
| 215 | 58412.9288 | 0.0020 | -0.0212 | 31 |
| 216 | 58412.9909 | 0.0010 | -0.0195 | 41 |
| 282 | 58416.9813 | 0.0010 | -0.0120 | 41 |
| 375 | 58422.6029 | 0.0027 | -0.0004 | 69 |
| 415 | 58425.0282 | 0.0013 | 0.0115 | 34 |

**Table E2.** Times of superhump maxima in the 2018 outburst of EG Cnc.

| $E$ | Max† | Error | $O-C$‡ | $N$§ |
|---|---|---|---|---|
| 438 | 58426.4198 | 0.0017 | 0.0154 | 47 |
| 452 | 58427.2654 | 0.0013 | 0.0164 | 59 |
| 453 | 58427.3307 | 0.0015 | 0.0213 | 48 |
| 457 | 58427.5682 | 0.0010 | 0.0175 | 35 |
| 473 | 58428.5375 | 0.0015 | 0.0214 | 139 |
| 490 | 58429.5634 | 0.0011 | 0.0217 | 46 |
| 491 | 58429.6257 | 0.0011 | 0.0237 | 33 |
| 497 | 58429.9829 | 0.0008 | 0.0189 | 66 |
| 498 | 58430.0450 | 0.0023 | 0.0206 | 33 |
| 501 | 58430.2283 | 0.0016 | 0.0229 | 59 |
| 502 | 58430.2919 | 0.0023 | 0.0262 | 49 |
| 506 | 58430.5292 | 0.0011 | 0.0222 | 33 |
| 507 | 58430.5891 | 0.0013 | 0.0218 | 33 |
| 508 | 58430.6497 | 0.0022 | 0.0220 | 33 |
| 514 | 58431.0163 | 0.0014 | 0.0266 | 48 |
| 523 | 58431.5619 | 0.0012 | 0.0292 | 49 |
| 524 | 58431.6230 | 0.0021 | 0.0300 | 33 |
| 588 | 58435.4954 | 0.0013 | 0.0410 | 29 |
| 589 | 58435.5497 | 0.0013 | 0.0350 | 32 |
| 590 | 58435.6111 | 0.0023 | 0.0361 | 33 |
| 596 | 58435.9751 | 0.0011 | 0.0380 | 51 |
| 597 | 58436.0319 | 0.0008 | 0.0345 | 50 |
| 607 | 58436.6362 | 0.0016 | 0.0355 | 90 |
| 608 | 58436.6917 | 0.0013 | 0.0307 | 85 |
| 612 | 58436.9397 | 0.0009 | 0.0373 | 33 |
| 613 | 58436.9915 | 0.0007 | 0.0288 | 48 |
| 629 | 58437.9563 | 0.0008 | 0.0283 | 47 |
| 635 | 58438.3119 | 0.0013 | 0.0219 | 82 |
| 656 | 58439.5941 | 0.0009 | 0.0370 | 144 |
| 657 | 58439.6557 | 0.0012 | 0.0384 | 118 |
| 680 | 58441.0389 | 0.0012 | 0.0339 | 43 |
| 687 | 58441.4534 | 0.0012 | 0.0260 | 16 |
| 718 | 58443.3419 | 0.0011 | 0.0442 | 66 |
| 866 | 58452.2698 | 0.0032 | 0.0427 | 28 |
| 867 | 58452.3347 | 0.0017 | 0.0474 | 36 |
| 870 | 58452.5147 | 0.0012 | 0.0463 | 33 |
| 871 | 58452.5753 | 0.0011 | 0.0466 | 33 |
| 887 | 58453.5367 | 0.0009 | 0.0426 | 34 |
| 888 | 58453.5987 | 0.0011 | 0.0443 | 76 |
| 889 | 58453.6585 | 0.0012 | 0.0438 | 49 |
| 954 | 58457.5860 | 0.0009 | 0.0496 | 26 |
| 955 | 58457.6450 | 0.0013 | 0.0483 | 33 |
| 972 | 58458.6740 | 0.0018 | 0.0516 | 43 |
| 1004 | 58460.6090 | 0.0006 | 0.0560 | 38 |
| 1058 | 58463.8709 | 0.0033 | 0.0599 | 50 |
| 1059 | 58463.9327 | 0.0017 | 0.0613 | 46 |
| 1153 | 58469.6120 | 0.0008 | 0.0693 | 38 |
| 1154 | 58469.6726 | 0.0007 | 0.0696 | 41 |
| 1187 | 58471.6696 | 0.0008 | 0.0756 | 75 |

*Cycle counts.

†BJD−2400000.0.

‡ C = 2458399.9709+0.06033338 E.

§Number of points used for determining the maximum.
